# Supplementary material for: When Reasoning Meets Information Aggregation: A Case Study with Sports Narratives
Source: arXiv:2406.12084 source file (2024-10-04)
Supplement: Supplementary file 1 [file Appendix.tex]

\section{Appendix}
\label{ssec: appendix}

\subsection{Experiments on Claude-3-Opus}

Anthropic release it's most advance LLM, Claude-3-Opus on march 2024 ~\citep{claude-3}. We conducted comprehensive reasoning experiments on sport analytics and present model-wise comparison in this section.

\begin{figure}[h]
\centering
\includegraphics[width=1\linewidth]{figures/claude-3_radar.pdf}
\caption{\small Both results of NBA and NFL sport are presented in above chart. In this figure, we normalized the value of accuracy with maximum score and present performance comparison with Claude-2.1 and GPT-4. Claude-3-Opus exhibits similar results on par with Claude-2.1, indicating our proposed task remains challenge even for the most-advanced LLMs.}
\label{fig:claude3}
\end{figure}

\subsection{Hallucinated Responses}
\label{ssec: hallucination}

\begin{figure}[h]
\centering
\includegraphics[width=0.8\linewidth,height=5cm]{figures/hallucination.pdf}
\caption{\small Hallucinated response when task contains only one sport description (step\_size=1)}
\label{fig:hall-llama2}
\end{figure}

We addressed one particular type of hallucination is overestimation of scores as shown in \ref{fig:hall-llama2}. 

We analyze model outputs from NBA divide-and-conquer experiments. Once the model’s prediction exceeds the threshold, defined by maximum points gained in ground truth at a certain step size, we identify it as hallucinations. We found that Llama-2-70b exhibited a significant error rate of \textbf{46.84\%} at step size = 1 which directly results in oddly high MAPE as we presented in Table \ref{tab: NBA results}. The close-source models responsed with fewer than 1\% of hallucinations.

\begin{figure}[h]
\centering
\includegraphics[width=1\linewidth]{figures/hall-team-predict.pdf}
%\vspace{-0.05in}
\caption{\small LLMs predict a team name when player and team identities were masked.}
\label{fig:hall-team}
\end{figure}
When we assessing the impacts of related sports information, an unusual response caught our attention as presented in Figure \ref{fig:hall-team}. In this task, all teams and player should be masked out. But LLMs includes GPT-3.5, Claude-2.1 and Llama2-70b predict a team name in their responses and reasoning based on it. In analysis results from Table \ref{tab: related information}, those models present a close or even better reasoning performance over natural game input. Meanwhile, other models, GPT-4 and Gemini-Pro, which didn't predict related sports information shows a great performance degradation.

\subsection{Instruction Following Verification}
\input{tables/cot_error_responses}

\begin{figure}[h]
\centering
\includegraphics[width=1\linewidth, height=10cm]{figures/gemini-cot-exp.pdf}
%\vspace{-0.05in}
\caption{\small Example from HalfGame reasoning task with CoT instruction. Gemini-Pro is the only model respond with Python script. We regard this as error presentation of middle steps since it does not showing the math reasoning procedure.}
\label{fig:gemini-cot-exp}
\end{figure}

The content in Table \ref{tab: error_cot} is an example of a common error response occurred when we use CoT method. We present another type of error response in Figure \ref{fig:gemini-cot-exp}. Finally, We post the overall accuracy comparison across all tasks whichever requires JSON formatting or CoT instruction following capability in Figure \ref{fig:nba-inst-following} and Figure \ref{fig:nfl-inst-following}.

\begin{figure*}[h]
\centering
\includegraphics[width=1\linewidth, height=7cm]{figures/NBA_inst_following.pdf}
%\vspace{-0.05in}
\caption{\small Instruction following accuracy bar chart for NBA tasks. We calculated number of non-zero digits in the response to assess whether LLM perform step-by-step reasoning process. For NBA tasks, we set 10 as threshold and we analyze the model's instruction following ability through trends.}
\label{fig:nba-inst-following}
\end{figure*}

\begin{figure*}[h]
\centering
\includegraphics[width=1\linewidth, height=8cm]{figures/NFL_inst_following.pdf}
%\vspace{-0.05in}
\caption{\small Instruction following accuracy bar chart for NFL tasks. We applied same justification method for CoT accuracy. For NFL tasks, we set 6 as threshold because less scoring moves included in game input.}
\label{fig:nfl-inst-following}
\end{figure*}
